# Supplementary material for: A Unified Hyperparameter Optimization Pipeline for Transformer-Based Time Series Forecasting Models
Source: arXiv:2501.01394 source file (2025-01-02)
Supplement: Supplementary file 1 [file 6_appendix.tex]

\newpage
\appendix
\section{Dataset}
% \begin{table}[!ht]
%     \centering
%     \caption{Summary of four datasets.}
%     \label{dataset}
%     \begin{tabular}{c|c|c|c|c}
%     % \hline
%      \hline
%         Datasets & ETTh1 & Weather & Electricity & Traffic \\ 
%         \hline
%         Variables & 7 & 21 & 321 & 862 \\ 
%         \hline
%         Timesteps & 17420 & 52696 & 26304 & 17544 \\
%     \hline
%     \end{tabular}
% \end{table}
\section{Parameters}
\subsection{Default Parameters}
\begin{table*}[!ht]
\caption{Major Parameters in the Time Series Library}
\label{Maj_parameters}
\centering
\resizebox{\textwidth}{!}{
\begin{tabular}{c | c | c | l}
\hline
\textbf{Parameter} & \textbf{Module}                   & \textbf{Default}       & \textbf{Help}   \\
\hline
task\_name         & \# basic config                   & 'long\_term\_forecast' & task name, options:{[}long\_term\_forecast, short\_term\_forecast, imputation, classification, anomaly\_detection{]} \\
is\_training       & \# basic config                   & 1                      & status                                                                                                               \\
model\_id          & \# basic config                   & 'test'                 & model id                                                                                                             \\
model              & \# basic config                   & 'Autoformer'           & model name, options: {[}Autoformer,  Transformer,  TimesNet{]}                                                       \\
data               & \# data loader                    & 'ETTm1'                & dataset type                                                                                                         \\
root\_path         & \# data loader                    & './data/ETT/'          & root path of the data file                                                                                           \\
data\_path         & \# data loader                    & 'ETTh1.csv'            & data file                                                                                                            \\
features           & \# data loader                    & 'M'                    & forecasting task, options:{[}M, S,  MS{]}; M:multivariate predict multivariate,                                      \\
                   &                                   &                        & S:univariate predict univariate, MS:multivariate predict univariate                                                  \\
target             & \# data loader                    & 'OT'                   & target feature in S or MS task                                                                                       \\
freq               & \# data loader                    & 'h'                    & freq for time features encoding, options:{[}s:secondly, t:minutely, h:hourly, d:daily,                               \\
                   &                                   &                        & b:business days, w:weekly, m:monthly{]},  you can also use more detailed freq like 15min or 3h                       \\
checkpoints        & \# data loader                    & './checkpoints/'       & location of model checkpoints                                                                                        \\
seq\_len           & \# forecasting task               & 96                     & input sequence length                                                                                                \\
label\_len         & \# forecasting task               & 48                     & start token length                                                                                                   \\
pred\_len          & \# forecasting task               & 96                     & prediction sequence length                                                                                           \\
seasonal\_patterns & \# forecasting task               & 'Monthly'              & subset for M4                                                                                                        \\
inverse            & \# forecasting task               & FALSE                  & inverse output data                                                                                                  \\
mask\_rate         & \# inputation task                & 0.25                   & mask ratio                                                                                                           \\
anomaly\_ratio     & \# anomaly detection task         & 0.25                   & prior anomaly ratio (\%)                                                                                             \\
top\_k             & \# model define                   & 5                      & for TimesBlock                                                                                                       \\
num\_kernels       & \# model define                   & 6                      & for Inception                                                                                                        \\
enc\_in            & \# model define                   & 7                      & encoder input size                                                                                                   \\
dec\_in            & \# model define                   & 7                      & decoder input size                                                                                                   \\
c\_out             & \# model define                   & 7                      & output size                                                                                                          \\
d\_model           & \# model define                   & 512                    & dimension of model                                                                                                   \\
n\_heads           & \# model define                   & 8                      & num of heads                                                                                                         \\
e\_layers          & \# model define                   & 2                      & num of encoder layers                                                                                                \\
d\_layers          & \# model define                   & 1                      & num of decoder layers                                                                                                \\
d\_ff              & \# model define                   & 2048                   & dimension of fcn                                                                                                     \\
moving\_avg        & \# model define                   & 25                     & window size of moving average                                                                                        \\
factor             & \# model define                   & 1                      & attn factor                                                                                                          \\
distil             & \# model define                   & TRUE                   & whether to use distilling in encoder using this argument means not using distilling                                  \\
dropout            & \# model define                   & 0.1                    & dropout                                                                                                              \\
embed              & \# model define                   & 'timeF'                & time features encoding  options:{[}timeF,  fixed,  learned{]}                                                        \\
activation         & \# model define                   & 'gelu'                 & activation                                                                                                           \\
output\_attention  & \# model define                   & TRUE                   & whether to output attention in ecoder                                                                                \\
num\_workers       & \# optimization                   & 10                     & data loader num workers                                                                                              \\
itr                & \# optimization                   & 1                      & experiments times                                                                                                    \\
train\_epochs      & \# optimization                   & 10                     & train epochs                                                                                                         \\
batch\_size        & \# optimization                   & 32                     & batch size of train input data                                                                                       \\
patience           & \# optimization                   & 3                      & early stopping patience                                                                                              \\
learning\_rate     & \# optimization                   & 0.0001                 & optimizer learning rate                                                                                              \\
des                & \# optimization                   & 'test'                 & exp description                                                                                                      \\
loss               & \# optimization                   & 'MSE'                  & loss function                                                                                                        \\
lradj              & \# optimization                   & 'type1'                & adjust learning rate                                                                                                 \\
use\_amp           & \# optimization                   & FALSE                  & use automatic mixed precision training                                                                               \\
use\_gpu           & \# GPU                            & TRUE                   & use gpu                                                                                                              \\
gpu                & \# GPU                            & 0                      & gpu                                                                                                                  \\
use\_multi\_gpu    & \# GPU                            & FALSE                  & use multiple gpus                                                                                                    \\
devices            & \# GPU                            & '0,1,2,3'              & device ids of multile gpus                                                                                           \\
p\_hidden\_dims    & \# de-stationary projector params & {[}128,128{]}          & hidden layer dimensions of projector (List                                                                           \\
p\_hidden\_layers  & \# de-stationary projector params & 2                      & number of hidden layers in projector        \\
\hline
\end{tabular}
}
\end{table*}

\newpage
\subsection{Parameters for Different Models}
